# Supplementary material for: Coupling Quantum Dots to Elastic Waves in a Phononic Crystal Waveguide
Source: arXiv:2601.14162 source file (2026-01-20)
Supplement: Supplementary file 1 [file dipoles_tables.pdf]

# **Supplementary Material: Dipole Moments**

GaAs and InAs Quantum Dots

Directions:  $x = [110]$ ,  $y = [\bar{1}10]$ ,  $z = [001]$   
Units: Electric field [kV/cm], Dipole [nm·e]

# GaAs Quantum Dot

| $\mathcal{E}_x$ | $\mathcal{E}_y$ | $\mathcal{E}_z$ | $p_x$    | $p_y$    | $p_z$   |
|-----------------|-----------------|-----------------|----------|----------|---------|
| -20.0           | 0.0             | 0.0             | -17.1260 | -0.1112  | 0.3847  |
| -10.0           | 0.0             | 0.0             | -6.2436  | -0.0379  | 0.0285  |
| -5.0            | 0.0             | 0.0             | -2.4933  | -0.0075  | -0.0553 |
| -2.0            | 0.0             | 0.0             | -0.9320  | 0.0034   | -0.0634 |
| -1.0            | 0.0             | 0.0             | -0.4647  | 0.0058   | -0.0644 |
| -0.5            | 0.0             | 0.0             | -0.2329  | 0.0068   | -0.0647 |
| 0.0             | 0.0             | 0.0             | -0.0013  | 0.0077   | -0.0649 |
| 0.5             | 0.0             | 0.0             | 0.2303   | 0.0085   | -0.0649 |
| 1.0             | 0.0             | 0.0             | 0.4624   | 0.0092   | -0.0647 |
| 2.0             | 0.0             | 0.0             | 0.9309   | 0.0107   | -0.0640 |
| 5.0             | 0.0             | 0.0             | 2.5017   | 0.0151   | -0.0554 |
| 10.0            | 0.0             | 0.0             | 6.2405   | 0.0277   | 0.0293  |
| 20.0            | 0.0             | 0.0             | 17.0516  | 0.0959   | 0.3614  |
| 0.0             | -20.0           | 0.0             | -0.1180  | -17.2250 | 0.4248  |
| 0.0             | -10.0           | 0.0             | -0.0161  | -5.8431  | 0.0344  |
| 0.0             | -5.0            | 0.0             | -0.0081  | -2.3948  | -0.0497 |
| 0.0             | -2.0            | 0.0             | -0.0049  | -0.8849  | -0.0625 |
| 0.0             | -1.0            | 0.0             | -0.0032  | -0.4337  | -0.0642 |
| 0.0             | -0.5            | 0.0             | -0.0023  | -0.2124  | -0.0646 |
| 0.0             | 0.0             | 0.0             | -0.0013  | 0.0077   | -0.0649 |
| 0.0             | 0.5             | 0.0             | -0.0003  | 0.2276   | -0.0649 |
| 0.0             | 1.0             | 0.0             | 0.0009   | 0.4487   | -0.0647 |
| 0.0             | 2.0             | 0.0             | 0.0033   | 0.8989   | -0.0636 |
| 0.0             | 5.0             | 0.0             | 0.0122   | 2.3960   | -0.0530 |
| 0.0             | 10.0            | 0.0             | 0.0347   | 5.7829   | 0.0229  |
| 0.0             | 20.0            | 0.0             | 0.2103   | 17.4899  | 0.4288  |
| 0.0             | 0.0             | -20.0           | -0.0032  | 0.0120   | -0.6983 |
| 0.0             | 0.0             | -10.0           | -0.0023  | 0.0098   | -0.3816 |
| 0.0             | 0.0             | -5.0            | -0.0018  | 0.0087   | -0.2230 |
| 0.0             | 0.0             | -2.0            | -0.0015  | 0.0081   | -0.1280 |
| 0.0             | 0.0             | -1.0            | -0.0014  | 0.0079   | -0.0964 |
| 0.0             | 0.0             | -0.5            | -0.0014  | 0.0078   | -0.0807 |
| 0.0             | 0.0             | 0.0             | -0.0013  | 0.0077   | -0.0649 |
| 0.0             | 0.0             | 0.5             | -0.0013  | 0.0076   | -0.0491 |
| 0.0             | 0.0             | 1.0             | -0.0012  | 0.0075   | -0.0333 |
| 0.0             | 0.0             | 2.0             | -0.0011  | 0.0073   | -0.0018 |
| 0.0             | 0.0             | 5.0             | -0.0008  | 0.0066   | 0.0924  |
| 0.0             | 0.0             | 10.0            | -0.0004  | 0.0056   | 0.2485  |
| 0.0             | 0.0             | 20.0            | 0.0005   | 0.0037   | 0.5558  |

# InAs Quantum Dot

| $\mathcal{E}_x$ | $\mathcal{E}_y$ | $\mathcal{E}_z$ | $p_x$   | $p_y$   | $p_z$   |
|-----------------|-----------------|-----------------|---------|---------|---------|
| -20.0           | 0.0             | 0.0             | -5.5912 | 0.0000  | -0.2593 |
| -10.0           | 0.0             | 0.0             | -2.6492 | 0.0000  | -0.1834 |
| -5.0            | 0.0             | 0.0             | -1.3004 | 0.0000  | -0.1678 |
| -2.0            | 0.0             | 0.0             | -0.5172 | 0.0000  | -0.1639 |
| -1.0            | 0.0             | 0.0             | -0.2584 | 0.0000  | -0.1634 |
| -0.5            | 0.0             | 0.0             | -0.1292 | 0.0000  | -0.1632 |
| 0.0             | 0.0             | 0.0             | -0.0000 | 0.0000  | -0.1632 |
| 0.5             | 0.0             | 0.0             | 0.1292  | 0.0000  | -0.1632 |
| 1.0             | 0.0             | 0.0             | 0.2584  | 0.0000  | -0.1634 |
| 2.0             | 0.0             | 0.0             | 0.5172  | 0.0000  | -0.1639 |
| 5.0             | 0.0             | 0.0             | 1.3004  | 0.0000  | -0.1678 |
| 10.0            | 0.0             | 0.0             | 2.6492  | 0.0000  | -0.1834 |
| 20.0            | 0.0             | 0.0             | 5.5912  | 0.0000  | -0.2593 |
| 0.0             | -20.0           | 0.0             | -0.0000 | -6.5594 | -0.2204 |
| 0.0             | -10.0           | 0.0             | -0.0000 | -2.9734 | -0.1741 |
| 0.0             | -5.0            | 0.0             | -0.0000 | -1.4424 | -0.1655 |
| 0.0             | -2.0            | 0.0             | -0.0000 | -0.5718 | -0.1636 |
| 0.0             | -1.0            | 0.0             | -0.0000 | -0.2855 | -0.1633 |
| 0.0             | -0.5            | 0.0             | -0.0000 | -0.1427 | -0.1632 |
| 0.0             | 0.0             | 0.0             | -0.0000 | 0.0000  | -0.1632 |
| 0.0             | 0.5             | 0.0             | -0.0000 | 0.1427  | -0.1632 |
| 0.0             | 1.0             | 0.0             | -0.0000 | 0.2856  | -0.1633 |
| 0.0             | 2.0             | 0.0             | -0.0000 | 0.5718  | -0.1636 |
| 0.0             | 5.0             | 0.0             | -0.0000 | 1.4424  | -0.1655 |
| 0.0             | 10.0            | 0.0             | -0.0000 | 2.9734  | -0.1741 |
| 0.0             | 20.0            | 0.0             | -0.0000 | 6.5594  | -0.2204 |
| 0.0             | 0.0             | -20.0           | -0.0000 | 0.0000  | -0.2883 |
| 0.0             | 0.0             | -10.0           | -0.0000 | 0.0000  | -0.2259 |
| 0.0             | 0.0             | -5.0            | -0.0000 | 0.0000  | -0.1946 |
| 0.0             | 0.0             | -2.0            | -0.0000 | 0.0000  | -0.1758 |
| 0.0             | 0.0             | -1.0            | -0.0000 | 0.0000  | -0.1695 |
| 0.0             | 0.0             | -0.5            | -0.0000 | 0.0000  | -0.1663 |
| 0.0             | 0.0             | 0.0             | -0.0000 | 0.0000  | -0.1632 |
| 0.0             | 0.0             | 0.5             | -0.0000 | 0.0000  | -0.1601 |
| 0.0             | 0.0             | 1.0             | -0.0000 | 0.0000  | -0.1569 |
| 0.0             | 0.0             | 2.0             | -0.0000 | 0.0000  | -0.1506 |
| 0.0             | 0.0             | 5.0             | -0.0000 | 0.0000  | -0.1317 |
| 0.0             | 0.0             | 10.0            | -0.0000 | 0.0000  | -0.1001 |
| 0.0             | 0.0             | 20.0            | -0.0000 | 0.0000  | -0.0367 |
