# Supplementary material for: Coupling Quantum Dots to Elastic Waves in a Phononic Crystal Waveguide
Source: arXiv:2601.14162 source file (2026-01-20)
Supplement: Supplementary file 2 [file quadrupoles_tables.pdf]

# **Supplementary Material: Quadrupole Tensors**

GaAs and InAs Quantum Dots

Directions:  $x = [110]$ ,  $y = [\bar{1}10]$ ,  $z = [001]$   
Units: Electric field [kV/cm], Quadrupole [ $\text{nm}^2 \cdot e$ ]

# GaAs Quantum Dot

| $\mathcal{E}_x$ | $\mathcal{E}_y$ | $\mathcal{E}_z$ | $Q_{11}$ | $Q_{12}$ | $Q_{13}$ | $Q_{21}$ | $Q_{22}$ | $Q_{23}$ | $Q_{31}$ | $Q_{32}$ | $Q_{33}$ |
|-----------------|-----------------|-----------------|----------|----------|----------|----------|----------|----------|----------|----------|----------|
| -20.0           | 0.0             | 0.0             | 239.933  | 148.514  | -177.963 | 148.514  | -132.365 | -4.240   | -177.963 | -4.240   | -107.569 |
| -10.0           | 0.0             | 0.0             | 63.607   | 53.363   | -56.240  | 53.363   | -37.156  | -0.521   | -56.240  | -0.521   | -26.451  |
| -5.0            | 0.0             | 0.0             | 16.287   | 21.025   | -21.258  | 21.025   | -11.999  | 0.407    | -21.258  | 0.407    | -4.288   |
| -2.0            | 0.0             | 0.0             | 5.156    | 7.731    | -7.693   | 7.731    | -6.249   | 0.558    | -7.693   | 0.558    | 1.093    |
| -1.0            | 0.0             | 0.0             | 2.399    | 3.774    | -3.715   | 3.774    | -4.840   | 0.583    | -3.715   | 0.583    | 2.441    |
| -0.5            | 0.0             | 0.0             | 1.146    | 1.813    | -1.751   | 1.813    | -4.204   | 0.592    | -1.751   | 0.592    | 3.059    |
| 0.0             | 0.0             | 0.0             | -0.016   | -0.144   | 0.207    | -0.144   | -3.620   | 0.599    | 0.207    | 0.599    | 3.636    |
| 0.5             | 0.0             | 0.0             | -1.086   | -2.101   | 2.167    | -2.101   | -3.087   | 0.604    | 2.167    | 0.604    | 4.173    |
| 1.0             | 0.0             | 0.0             | -2.069   | -4.062   | 4.133    | -4.062   | -2.602   | 0.607    | 4.133    | 0.607    | 4.671    |
| 2.0             | 0.0             | 0.0             | -3.818   | -8.018   | 8.120    | -8.018   | -1.756   | 0.608    | 8.120    | 0.608    | 5.573    |
| 5.0             | 0.0             | 0.0             | -7.664   | -21.298  | 21.734   | -21.298  | -0.038   | 0.564    | 21.734   | 0.564    | 7.702    |
| 10.0            | 0.0             | 0.0             | 3.789    | -52.952  | 56.038   | -52.952  | -7.484   | -0.020   | 56.038   | -0.020   | 3.695    |
| 20.0            | 0.0             | 0.0             | 70.302   | -146.291 | 173.926  | -146.291 | -49.087  | -2.161   | 173.926  | -2.161   | -21.215  |
| 0.0             | -20.0           | 0.0             | -185.117 | 61.459   | -2.831   | 61.459   | 348.205  | -185.490 | -2.831   | -185.490 | -163.088 |
| 0.0             | -10.0           | 0.0             | -48.862  | 20.445   | -0.229   | 20.445   | 90.458   | -53.939  | -0.229   | -53.939  | -41.596  |
| 0.0             | -5.0            | 0.0             | -15.494  | 8.371    | 0.129    | 8.371    | 26.895   | -20.895  | 0.129    | -20.895  | -11.402  |
| 0.0             | -2.0            | 0.0             | -5.221   | 3.044    | 0.179    | 3.044    | 6.769    | -7.299   | 0.179    | -7.299   | -1.547   |
| 0.0             | -1.0            | 0.0             | -2.513   | 1.436    | 0.193    | 1.436    | 1.396    | -3.296   | 0.193    | -3.296   | 1.117    |
| 0.0             | -0.5            | 0.0             | -1.241   | 0.644    | 0.200    | 0.644    | -1.149   | -1.341   | 0.200    | -1.341   | 2.391    |
| 0.0             | 0.0             | 0.0             | -0.016   | -0.144   | 0.207    | -0.144   | -3.620   | 0.599    | 0.207    | 0.599    | 3.636    |
| 0.0             | 0.5             | 0.0             | 1.169    | -0.934   | 0.215    | -0.934   | -6.030   | 2.537    | 0.215    | 2.537    | 4.861    |
| 0.0             | 1.0             | 0.0             | 2.320    | -1.728   | 0.222    | -1.728   | -8.393   | 4.484    | 0.222    | 4.484    | 6.073    |
| 0.0             | 2.0             | 0.0             | 4.550    | -3.348   | 0.236    | -3.348   | -13.024  | 8.454    | 0.236    | 8.454    | 8.474    |
| 0.0             | 5.0             | 0.0             | 10.818   | -8.713   | 0.267    | -8.713   | -26.402  | 21.738   | 0.267    | 21.738   | 15.583   |
| 0.0             | 10.0            | 0.0             | 15.786   | -20.561  | 0.187    | -20.561  | -40.334  | 52.827   | 0.187    | 52.827   | 24.548   |
| 0.0             | 20.0            | 0.0             | -1.704   | -57.959  | 0.717    | -57.959  | -27.924  | 181.774  | 0.717    | 181.774  | 29.628   |
| 0.0             | 0.0             | -20.0           | 0.252    | -0.148   | 2.472    | -0.148   | -3.646   | 5.916    | 2.472    | 5.916    | 3.393    |
| 0.0             | 0.0             | -10.0           | 0.165    | -0.145   | 1.338    | -0.145   | -3.634   | 3.257    | 1.338    | 3.257    | 3.469    |
| 0.0             | 0.0             | -5.0            | 0.088    | -0.145   | 0.771    | -0.145   | -3.629   | 1.926    | 0.771    | 1.926    | 3.541    |
| 0.0             | 0.0             | -2.0            | 0.029    | -0.144   | 0.433    | -0.144   | -3.624   | 1.129    | 0.433    | 1.129    | 3.595    |
| 0.0             | 0.0             | -1.0            | 0.007    | -0.144   | 0.320    | -0.144   | -3.622   | 0.864    | 0.320    | 0.864    | 3.615    |
| 0.0             | 0.0             | -0.5            | -0.005   | -0.144   | 0.264    | -0.144   | -3.621   | 0.732    | 0.264    | 0.732    | 3.626    |
| 0.0             | 0.0             | 0.0             | -0.016   | -0.144   | 0.207    | -0.144   | -3.620   | 0.599    | 0.207    | 0.599    | 3.636    |
| 0.0             | 0.0             | 0.5             | -0.029   | -0.144   | 0.151    | -0.144   | -3.619   | 0.467    | 0.151    | 0.467    | 3.647    |
| 0.0             | 0.0             | 1.0             | -0.041   | -0.144   | 0.095    | -0.144   | -3.617   | 0.334    | 0.095    | 0.334    | 3.658    |
| 0.0             | 0.0             | 2.0             | -0.067   | -0.144   | -0.017   | -0.144   | -3.614   | 0.070    | -0.017   | 0.070    | 3.681    |
| 0.0             | 0.0             | 5.0             | -0.154   | -0.144   | -0.353   | -0.144   | -3.603   | -0.721   | -0.353   | -0.721   | 3.757    |
| 0.0             | 0.0             | 10.0            | -0.327   | -0.144   | -0.908   | -0.144   | -3.576   | -2.031   | -0.908   | -2.031   | 3.903    |
| 0.0             | 0.0             | 20.0            | -0.790   | -0.145   | -1.999   | -0.145   | -3.485   | -4.611   | -1.999   | -4.611   | 4.275    |

# InAs Quantum Dot

| $\mathcal{E}_x$ | $\mathcal{E}_y$ | $\mathcal{E}_z$ | $Q_{11}$ | $Q_{12}$ | $Q_{13}$ | $Q_{21}$ | $Q_{22}$ | $Q_{23}$ | $Q_{31}$ | $Q_{32}$ | $Q_{33}$ |
|-----------------|-----------------|-----------------|----------|----------|----------|----------|----------|----------|----------|----------|----------|
| -20.0           | 0.0             | 0.0             | 53.305   | 10.064   | 17.195   | 10.064   | -24.359  | 0.467    | 17.195   | 0.467    | -28.946  |
| -10.0           | 0.0             | 0.0             | 26.360   | 4.768    | 7.981    | 4.768    | -9.987   | 0.330    | 7.981    | 0.330    | -16.373  |
| -5.0            | 0.0             | 0.0             | 19.162   | 2.341    | 4.044    | 2.341    | -6.278   | 0.302    | 4.044    | 0.302    | -12.884  |
| -2.0            | 0.0             | 0.0             | 16.301   | 0.931    | 1.783    | 0.931    | -4.830   | 0.295    | 1.783    | 0.295    | -11.471  |
| -1.0            | 0.0             | 0.0             | 15.545   | 0.465    | 1.037    | 0.465    | -4.450   | 0.294    | 1.037    | 0.294    | -11.096  |
| -0.5            | 0.0             | 0.0             | 15.201   | 0.233    | 0.665    | 0.233    | -4.277   | 0.294    | 0.665    | 0.294    | -10.924  |
| 0.0             | 0.0             | 0.0             | 14.880   | -0.000   | 0.294    | -0.000   | -4.117   | 0.294    | 0.294    | 0.294    | -10.764  |
| 0.5             | 0.0             | 0.0             | 14.581   | -0.233   | -0.078   | -0.233   | -3.967   | 0.294    | -0.078   | 0.294    | -10.614  |
| 1.0             | 0.0             | 0.0             | 14.305   | -0.465   | -0.449   | -0.465   | -3.829   | 0.294    | -0.449   | 0.294    | -10.475  |
| 2.0             | 0.0             | 0.0             | 13.818   | -0.931   | -1.193   | -0.931   | -3.588   | 0.295    | -1.193   | 0.295    | -10.230  |
| 5.0             | 0.0             | 0.0             | 12.920   | -2.341   | -3.440   | -2.341   | -3.157   | 0.302    | -3.440   | 0.302    | -9.763   |
| 10.0            | 0.0             | 0.0             | 13.644   | -4.768   | -7.321   | -4.768   | -3.629   | 0.330    | -7.321   | 0.330    | -10.015  |
| 20.0            | 0.0             | 0.0             | 26.467   | -10.064  | -16.262  | -10.064  | -10.940  | 0.467    | -16.262  | 0.467    | -15.527  |
| 0.0             | -20.0           | 0.0             | -3.365   | 11.807   | 0.397    | 11.807   | 31.958   | 17.858   | 0.397    | 17.858   | -28.593  |
| 0.0             | -10.0           | 0.0             | 9.788    | 5.352    | 0.313    | 5.352    | 6.387    | 7.977    | 0.313    | 7.977    | -16.175  |
| 0.0             | -5.0            | 0.0             | 12.876   | 2.596    | 0.298    | 2.596    | 0.008    | 4.012    | 0.298    | 4.012    | -12.884  |
| 0.0             | -2.0            | 0.0             | 14.156   | 1.029    | 0.294    | 1.029    | -2.647   | 1.768    | 0.294    | 1.768    | -11.509  |
| 0.0             | -1.0            | 0.0             | 14.528   | 0.514    | 0.294    | 0.514    | -3.407   | 1.030    | 0.294    | 1.030    | -11.121  |
| 0.0             | -0.5            | 0.0             | 14.707   | 0.257    | 0.294    | 0.257    | -3.768   | 0.662    | 0.294    | 0.662    | -10.939  |
| 0.0             | 0.0             | 0.0             | 14.880   | 0.000    | 0.294    | 0.000    | -4.116   | 0.294    | 0.294    | 0.294    | -10.764  |
| 0.0             | 0.5             | 0.0             | 15.049   | -0.257   | 0.294    | -0.257   | -4.453   | -0.074   | 0.294    | -0.074   | -10.596  |
| 0.0             | 1.0             | 0.0             | 15.214   | -0.514   | 0.294    | -0.514   | -4.778   | -0.442   | 0.294    | -0.442   | -10.436  |
| 0.0             | 2.0             | 0.0             | 15.528   | -1.029   | 0.294    | -1.029   | -5.392   | -1.179   | 0.294    | -1.179   | -10.136  |
| 0.0             | 5.0             | 0.0             | 16.338   | -2.596   | 0.298    | -2.596   | -6.916   | -3.416   | 0.298    | -3.416   | -9.422   |
| 0.0             | 10.0            | 0.0             | 16.924   | -5.352   | 0.313    | -5.352   | -7.885   | -7.350   | 0.313    | -7.350   | -9.039   |
| 0.0             | 20.0            | 0.0             | 12.377   | -11.807  | 0.397    | -11.807  | 0.473    | -17.065  | 0.397    | -17.065  | -12.851  |
| 0.0             | 0.0             | -20.0           | 16.489   | 0.000    | 0.519    | 0.000    | -3.191   | 0.519    | 0.519    | 0.519    | -13.299  |
| 0.0             | 0.0             | -10.0           | 15.672   | -0.000   | 0.407    | -0.000   | -3.645   | 0.407    | 0.407    | 0.407    | -12.027  |
| 0.0             | 0.0             | -5.0            | 15.273   | -0.000   | 0.350    | -0.000   | -3.879   | 0.350    | 0.350    | 0.350    | -11.394  |
| 0.0             | 0.0             | -2.0            | 15.037   | -0.000   | 0.316    | -0.000   | -4.021   | 0.316    | 0.316    | 0.316    | -11.016  |
| 0.0             | 0.0             | -1.0            | 14.958   | 0.000    | 0.305    | 0.000    | -4.069   | 0.305    | 0.305    | 0.305    | -10.890  |
| 0.0             | 0.0             | -0.5            | 14.919   | -0.000   | 0.299    | -0.000   | -4.093   | 0.299    | 0.299    | 0.299    | -10.827  |
| 0.0             | 0.0             | 0.0             | 14.880   | -0.000   | 0.294    | -0.000   | -4.117   | 0.294    | 0.294    | 0.294    | -10.764  |
| 0.0             | 0.0             | 0.5             | 14.841   | -0.000   | 0.288    | -0.000   | -4.140   | 0.288    | 0.288    | 0.288    | -10.701  |
| 0.0             | 0.0             | 1.0             | 14.803   | -0.000   | 0.282    | -0.000   | -4.165   | 0.282    | 0.282    | 0.282    | -10.638  |
| 0.0             | 0.0             | 2.0             | 14.725   | -0.000   | 0.271    | -0.000   | -4.213   | 0.271    | 0.271    | 0.271    | -10.512  |
| 0.0             | 0.0             | 5.0             | 14.494   | -0.000   | 0.237    | -0.000   | -4.358   | 0.237    | 0.237    | 0.237    | -10.136  |
| 0.0             | 0.0             | 10.0            | 14.113   | -0.000   | 0.180    | -0.000   | -4.604   | 0.180    | 0.180    | 0.180    | -9.509   |
| 0.0             | 0.0             | 20.0            | 13.369   | 0.000    | 0.066    | 0.000    | -5.106   | 0.066    | 0.066    | 0.066    | -8.263   |
